# Supplementary material for: On the Impact of the Communication Model on Realisability
Source: arXiv:2512.05609 source file (2025-12-05)
Supplement: Supplementary file 1 [file appendix-main.tex]

% !TEX root =  ../main.tex
%!TEX spellcheck = en_GB

%\section{Proof of Lemma~\ref{lem:pp-is-causally-closed}}
%\label{app:pp-is-causally-closed}

%\input{proofs/lem-pp-is-causally-closed.tex}

%\section{Proof of Proposition~\ref{prop:deadlock-free-as-a-property-on-mscs-for-p2p-and-synch}}
%\label{app:deadlock-free-as-a-property-on-mscs-for-p2p-and-synch}

%\propdeadlockfreeasapropertyonmscsforppandsynch*
%\input{proofs/prop-deadlock-free-as-a-property-on-mscs-for-p2p-and-synch.tex}

%\section{Proof of Theorem~\ref{thm:main-theorem-realisability}}
%\label{app:main-theorem-realisability}
%\maintheoremrealisability*
%\input{proofs/thm-main-theorem-implementability.tex}

%\section{Standard notions on automata}
%\label{app:automata-standards}
% \input{content/automata-standards.tex}

%\section{Proof of Lemma \ref{lem:pp-is-causally-closed}} \label{app:lemmacausallyclosed}
%\input{proofs/causallyclosed}

%\section{Proof of  Proposition \ref{prop:universal-existential-synch-inclusion}}\label{app:existuniversal}
%\universalesxistential*
%\input{proofs/existuniversal}

%\section{Proof of Lemma~\ref{lem:product-of-gt}}
%\label{app:product-of-gt}
%\lemproductofgt*
%\input{proofs/lem-product-of-gt.tex}

%\section{Proof of  Proposition \ref{prop:product-is-commutation-closed}}\label{app:productclosed}
%\productclosed*
%\input{proofs/productclosed}

%\section{Discussion about deadlock-free realizability and safe realizability}
%\label{app:discussion-deadlock-free-realizability-and-safe-realizability}
%\input{content/discussion-deadlock-free-realizability-and-safe-realizability.tex}
